# Supplementary material for: Time-Reversed Dissipation Induces Duality Between Minimizing Gradient Norm and Function Value
Source: arXiv:2305.06628 source file (2023-11-01)
Supplement: Supplementary file 1 [file Appendix_section1.tex]

\section{Omitted contents in \ref{sec::prior_works}}
XXX detailed prior works XXX
